# Supplementary material for: Mixed formulation of physics-informed neural networks for thermo-mechanically coupled systems and heterogeneous domains
Source: arXiv:2302.04954 source file (2023-09-06)
Supplement: Supplementary file 1 [file appendix_B.tex]

%%%%%%%%%%%%%%%%%%%%%%%%
\section{Appendix B: Simple example to clarify the importance of physical constraints in the training procedure}
In this example, we approximate a simple function via a standard neural network. First, we consider the following function $y(x)$ as the desired solution:
\begin{align}
\label{sol}
y(x) = \text{sin}(x) + 0.1~x + 0.1.
\end{align}
The above function is plotted as the reference (true) solution in Fig.~\ref{fig:data_phy}. next, this function is evaluated at $50$ points \textcolor{red}{true??} within the interval $x=[0,2]$. These points are referred to as data (sample) points and the training regime is highlighted via dark gray color in Fig.~\ref{fig:data_phy}.
A neural network with $4$ layers and $20$ neurons in each layer is then initialized. We used \emph{tanh} as an activation function for all the neurons. The loss function is defined as 
\begin{align}
\label{daaata}
\mathcal{L}_{data} =   
\text{MSE}\left(y_{o}(i)-y_{true}(i)\right).
\end{align}
By solely training the NN based on the given data points for 500 epochs, the orange curve is obtained (see also the gray region in Fig.~\ref{fig:losses_app}). This curve represents the true solution nicely in the training domain yet deviates from it for the points outside of the training regime.
\begin{figure}[H] 
  \centering
  \includegraphics[width=0.95\linewidth]{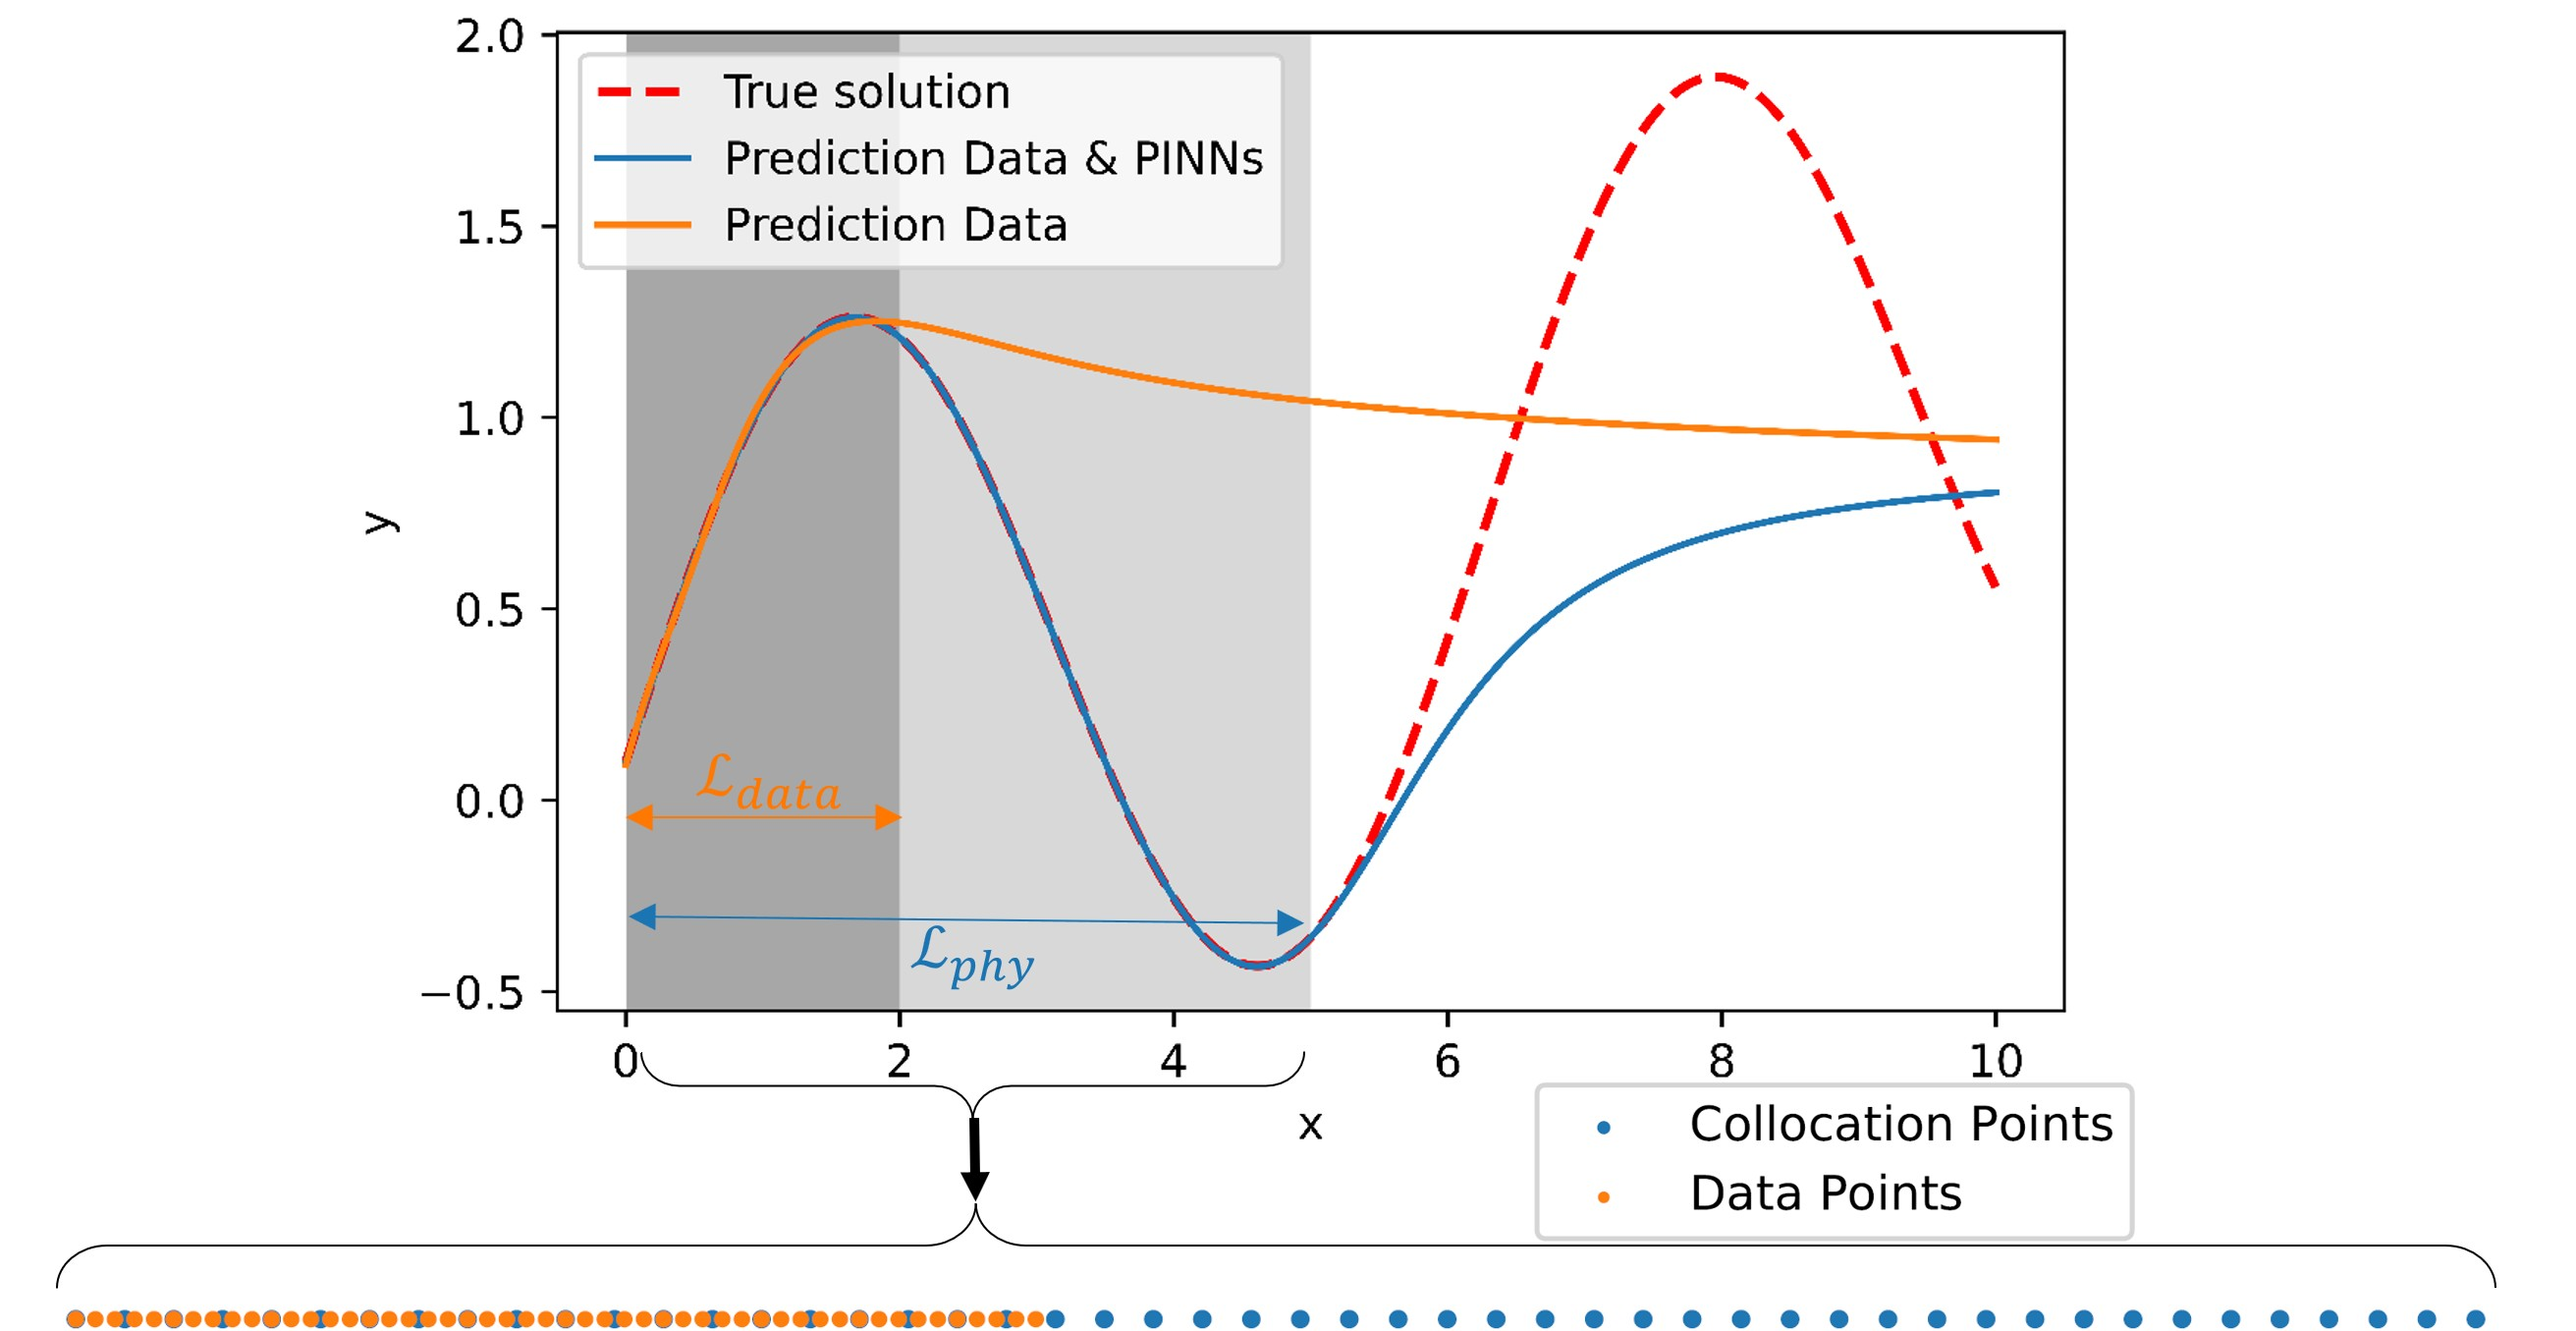}
  \caption{Obtained solution and accuracy of extrapolation from different approaches. }
  \label{fig:data_phy}
\end{figure}
Next, we construct a differential equate ion, by taking the first derivative of the relation in Eq.~\ref{sol} with respect to the parameter $x$. Therefore, we write the following 1st-order ordinary differential equation (ODE) subjected to the following boundary conditions:
\begin{align}
\label{def_1}
y'  &= \dfrac{\text{d}y}{\text{d}x} = \text{cos}(x) + 0.1,~~~y(0)=0.1,~~~y(5)=-0.358.
\end{align}
The idea is to utilize the relation in Eq.~\ref{def_1} as the governing equation for the target solution $y(x)$.
In other words, we intend to obtain (reproduce) the function $y(x)$, by feeding the above-mentioned ODE to the trained NN from the previous step which was based on pure data. Note that the same neural network with the same architecture and hyperparameters is again trained following the governing equation for another 500 epochs at the collocation point within the range $x=[0,5]$. See 50 blue collocation points as well as the light gray area in Fig.~\ref{fig:data_phy}. Moreover, the loss function for the second training part is plotted in blue in Fig.~\ref{fig:losses_app}. 
\begin{align}
\label{loss_ode_1}
\mathcal{L}_{phy} = 
\text{MSE}\left(\dfrac{\text{d}y_{o}}{\text{d}x} - \text{cos}(x) - 0.1 \right) + 
\text{MSE}\left(y_{o}(0)-0.1\right) + 
\text{MSE}\left(y_{o}(5)+0.358\right).
\end{align}
We conclude two points from the results in Fig.~\ref{fig:data_phy}. first, by employing the physical constraint beyond the sample data point and further training the NN, we can get more accurate results for a larger range beyond the initial sample points. Note that in physical simulations, there are some constraints that hold for any given condition. Next, it seems that if we test the NN performance beyond the range for the collocation points, the results might not still be reliable. In other words, the blue curve in Fig.~\ref{fig:data_phy} deviates from the dashed red one for $x=[5,10]$. Finally, one should also take into account the influence of other hyperparameters of the NN in the results for extrapolation. For example by proper choice for the activation function one has the chance to significantly improve the solution for the range beyond the data and collocation points. Further discussion on this point will be covered in future studies.
\begin{figure}[H] 
  \centering
  \includegraphics[width=0.7\linewidth]{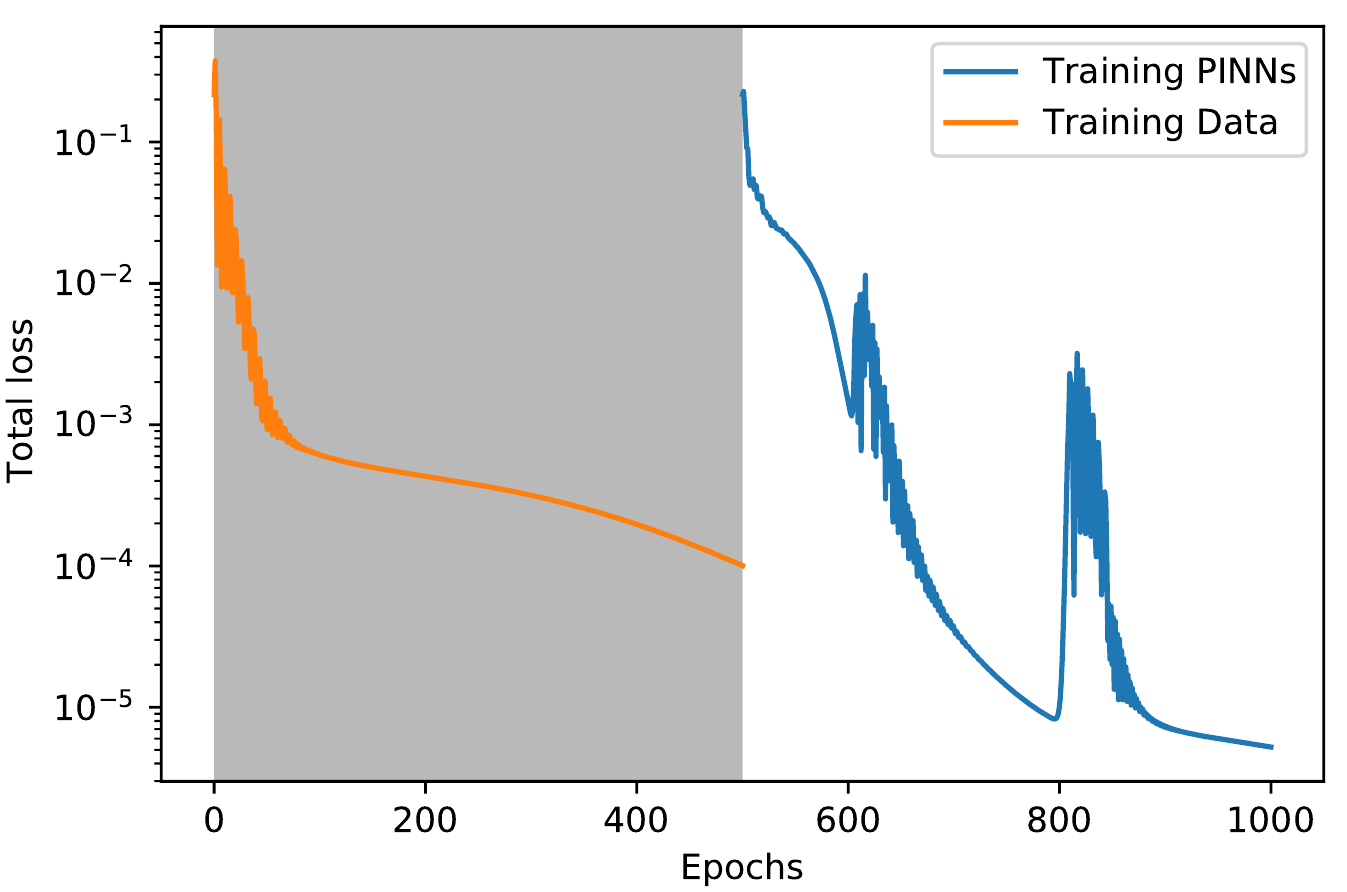}
  \caption{Loss function versus the number of epochs. After training with available data for 500 epochs, the network is further trained by means of the governing physical constraints for another 500 epochs.}
  \label{fig:losses_app}
\end{figure}
